# Supplementary material for: Pointing out the Shortcomings of Relation Extraction Models with Semantically Motivated Adversarials
Source: arXiv:2402.19076 source file (2024-02-29)
Supplement: Supplementary file 1 [file appendix.tex]

\begin{figure}[!ht]
    \centering
    \includegraphics[scale=0.27]{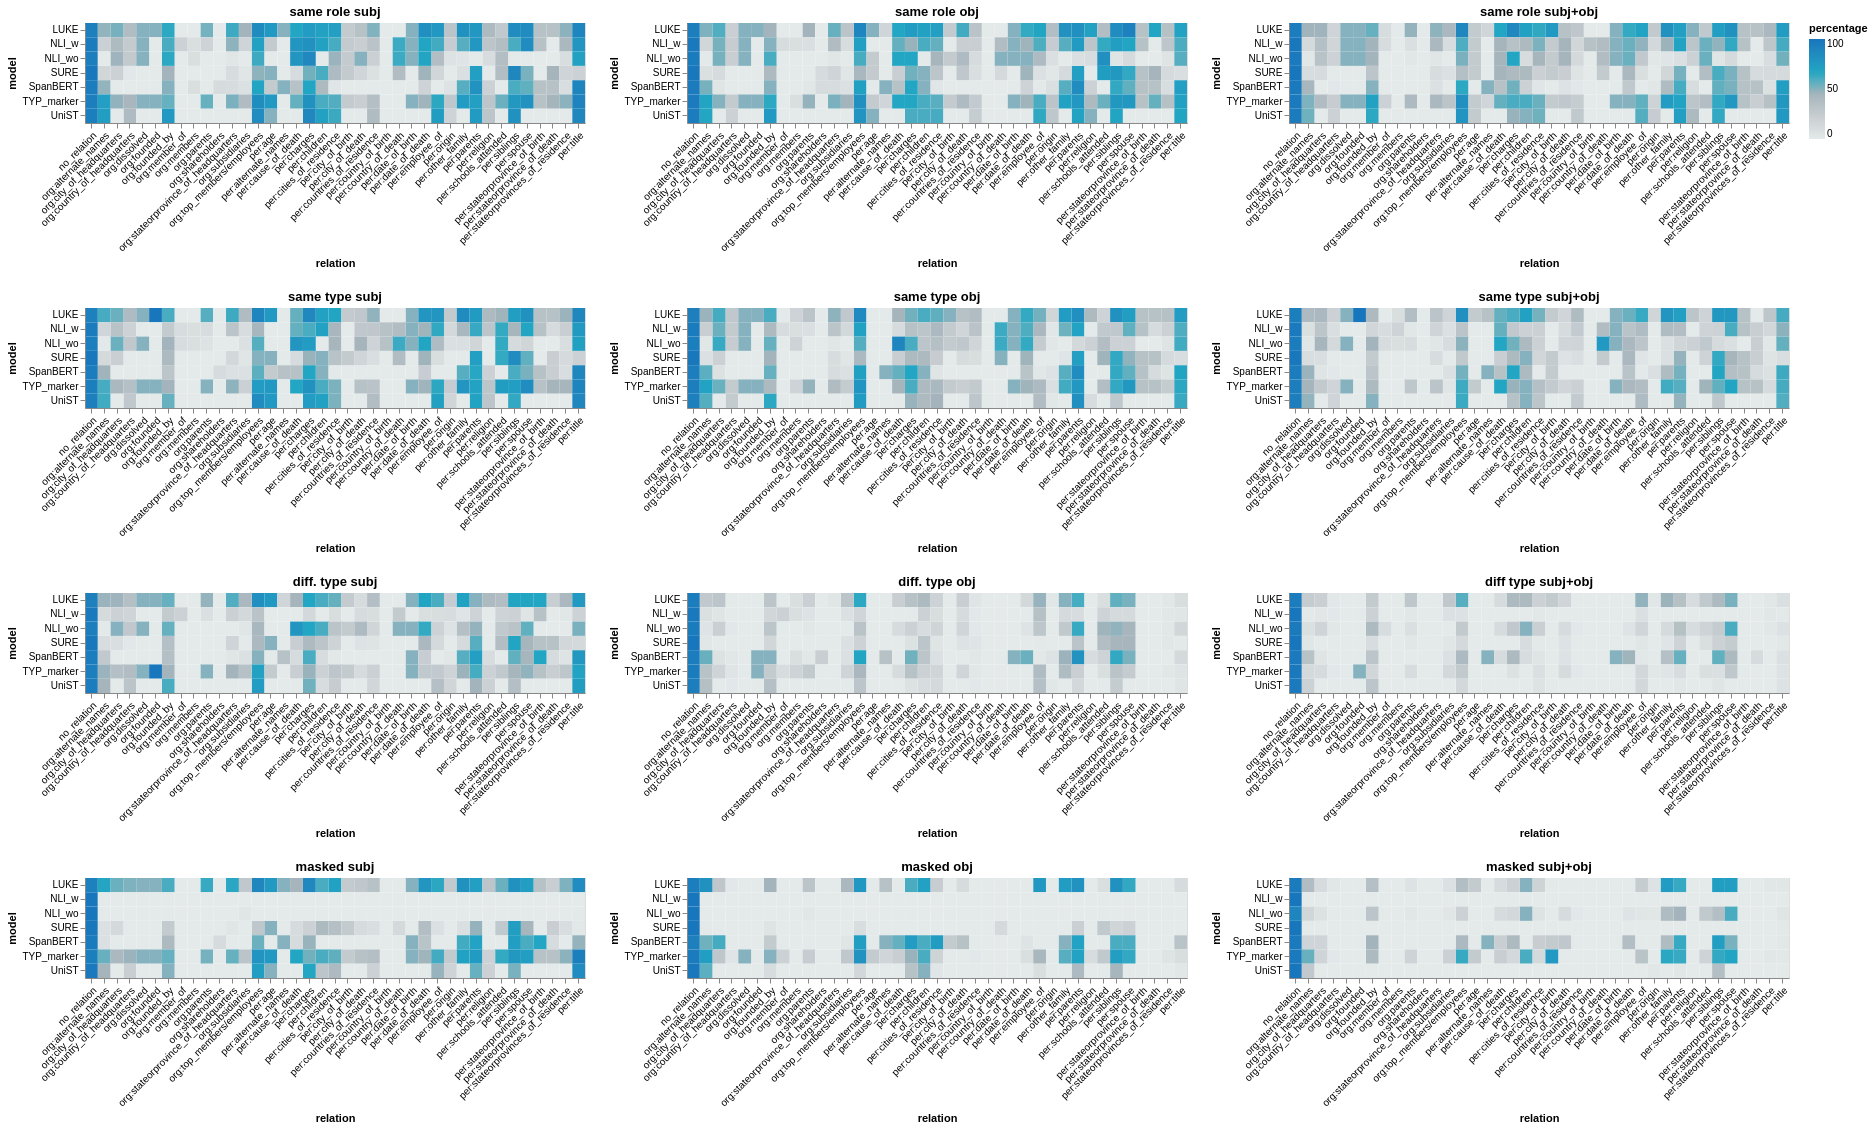}
    \caption{Relation-wise heatmap for every model, across all adversarial strategies}
    \label{fig:heatmap}
\end{figure}

\begin{figure}[!ht]
    \centering

    \includegraphics[scale=0.27]{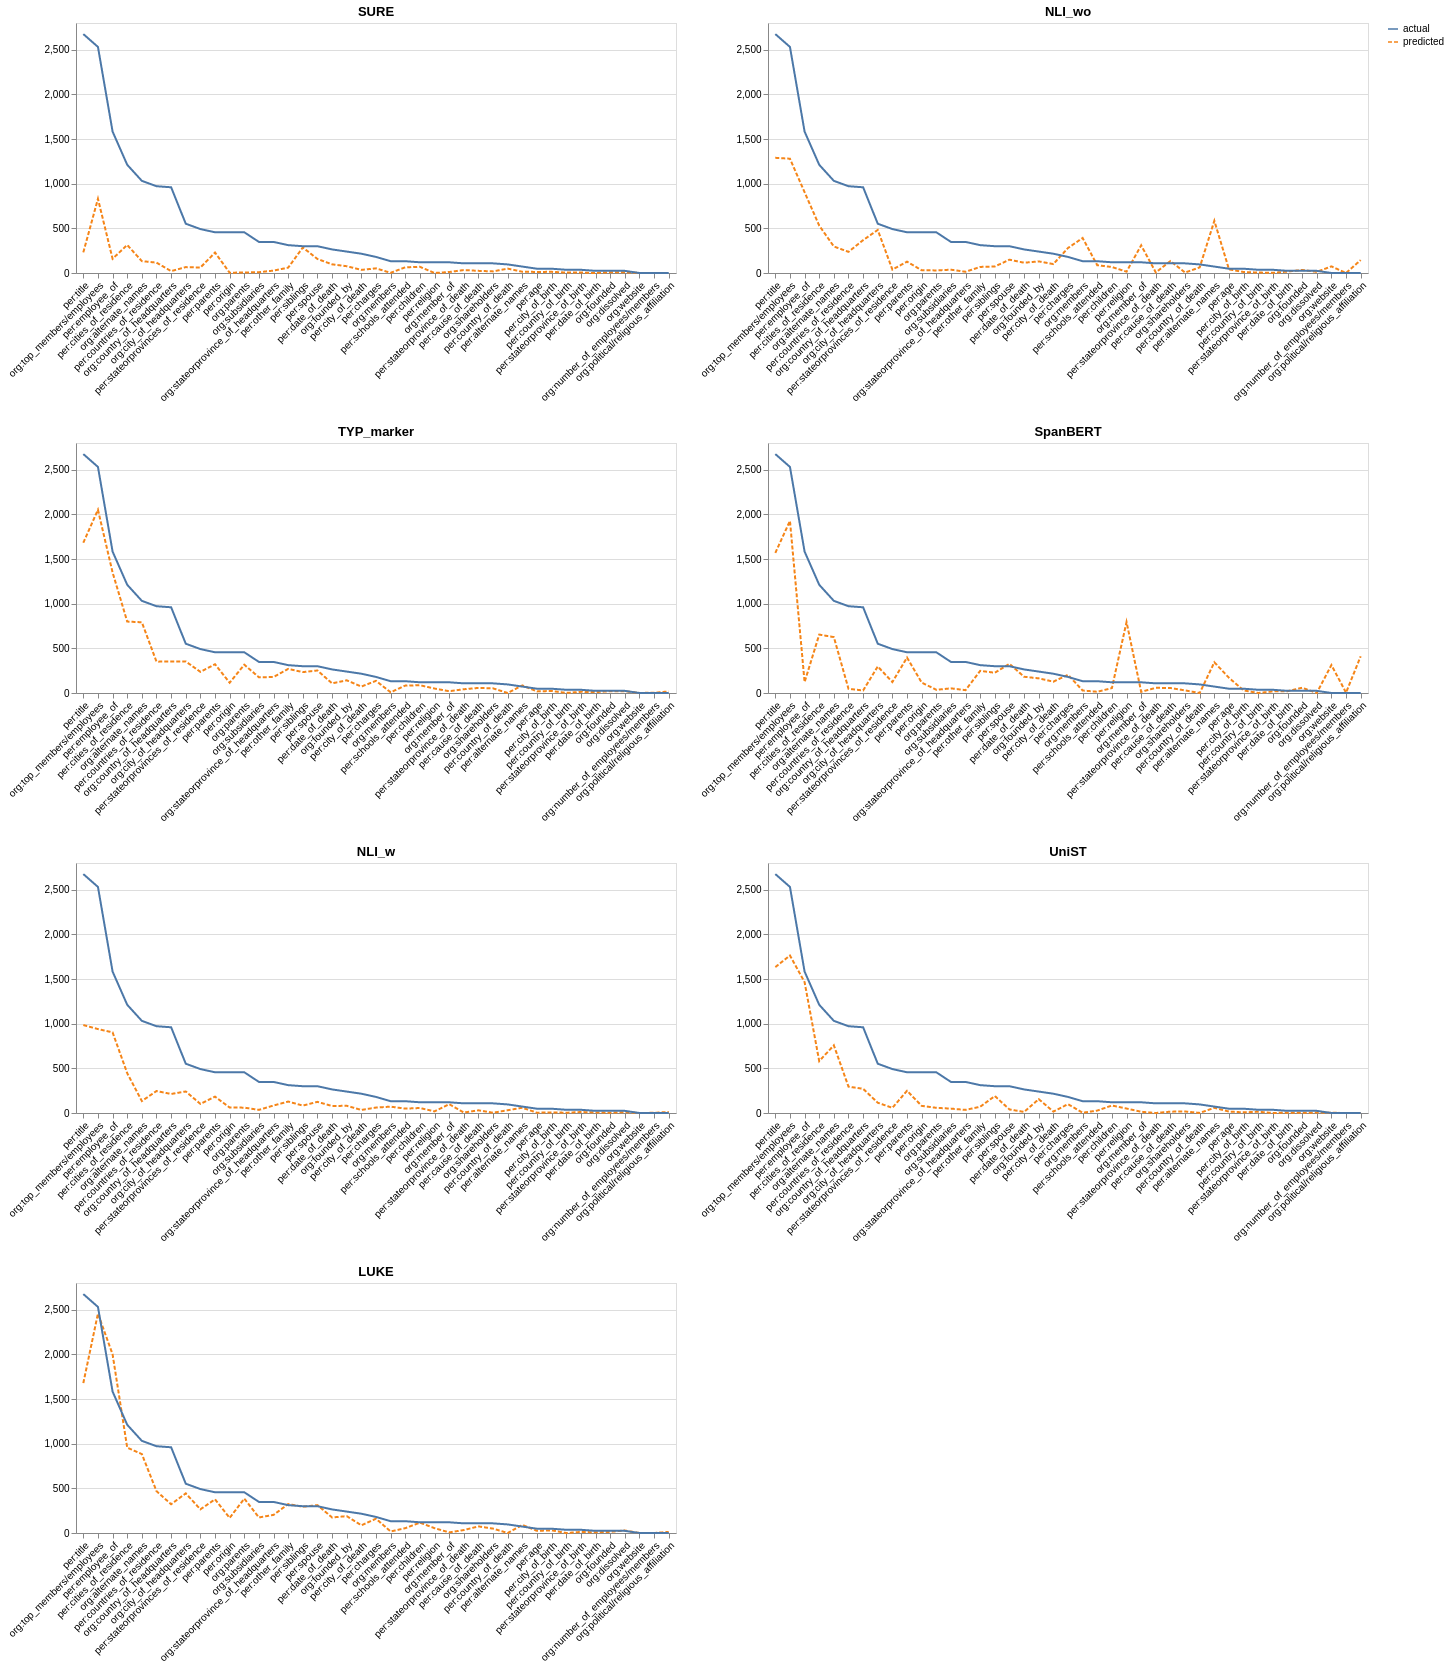}
     \caption{Absolute values of actual vs predicted relation labels for all the models across all adversarial sets ordered by the frequency of the relation label in the testing split. No\_relation was removed for better visualization}
    \label{fig:all_rels_all_models}
\end{figure*}
